# Supplementary material for: Provable Algorithms for Inference in Topic Models
Source: arXiv:1605.08491 source file (2016-05-27)
Supplement: Supplementary file 1 [file appendix.tex]

\begin{theorem}\label{thm:beyasian}
	Suppose an algorithm $\mathcal{A}$ that takes input $y$ and outputs %(random or deterministic) 
	$\mathcal A(y)$ satisfies that for any $x\in \mathcal{X}$, with probability $1-\delta^2$ over the randomness of $p_{y\vert x}$, it holds that
	\begin{equation}
		\|\mathcal A(y) - x\|\le \epsilon\,.\label{eqn:eqn1}
	\end{equation} 
	Then, for $1-\delta$ fraction of $y$ (with respect to marginal density $p_y$), it holds that the posterior distribution $x\vert y$ is concentrated in a $\epsilon$-ball $\mathcal B(\hat{x},\epsilon)$ for some $\hat{x}$. That is,  
	
	\begin{equation}
		\Pr_{y\vert x}[~\|\hat{x}-x\|\le \epsilon \mid y~]\ge 1-\delta\,.
	\end{equation}

\end{theorem}
